# Supplementary material for: New Constraints on Anisotropic Expansion from Supernovae Type Ia
Source: arXiv:2108.12497 source file (2022-04-28)
Supplement: Supplementary file 1 [file appendix-2.tex]

\section{Peculiar velocity covariance}

We can use the reconstructed velocity field to predict the velocity of the supernovae. However, there is no unique way to predict the peculiar velocity from the observations. Specifically, one can predict the peculiar velocity by integrating over a range of distances compatible with a supernova's distance estimate, or one can predict the peculiar velocity consistent with the observed redshift. In this work, we predict the velocity of the supernovae from the 2M++ reconstruction in the redshift space.

The 2M++ reconstruction employs linear perturbation theory to predict the velocities. As shown in \citet{10.1093/mnras/stv547}, this leads to an uncertainty of $\sigma_v = 150$ km/s. Therefore, assuming a Gaussian uncertainty, we can write the probability of the predicted redshift given the observed redshift as, 
\begin{equation}\label{eqn:p_cz}
    P(cz_{\text{pred}}(r)|cz_{\text{obs}}) = \frac{1}{\sqrt{2\pi\sigma^2_v}}\exp \bigg[-\frac{(cz_{\text{pred}} - cz_{\text{obs}})^2}{2\sigma^2_v} \bigg],
\end{equation}
where, 
\begin{equation}
    z_{\text{pred}}(r) = z_{\text{cos}}(r) + [1+z_{\text{cos}}(r)]\frac{V_r(r)}{c}.
\end{equation}
In the above equation, $z_{\text{cos}}$ is the cosmological redshift and  $V_r(r)$ is the radial component of the predicted peculiar velocity from 2M++. Using a variable transformation to write equation \eqref{eqn:p_cz} in terms of the comoving distance, $r$, we get, 
\begin{equation}\label{eqn:p_r}
    P(r|cz_{\text{obs}}) = P(cz_{\text{pred}}(r)|cz_{\text{obs}})\bigg|\frac{\partial cz_{\text{pred}}}{\partial r}\bigg|
\end{equation}
Note that the transformation between $r$ and $cz_{\text{pred}}$ may not be unique due to the existence of triple-valued regions. However, in practice, in our reconstruction, we checked that the reconstructed velocity field indeed leads to unique transformation between $r$ and $z_{\text{pred}}$ for the parameters under consideration. Nevertheless, it can lead to `flat' regions in redshift space (i.e, $\frac{\partial z_{\text{pred}}}{\partial r} \approx 0$), which can lead to large uncertainties in the predicted velocity. 

Using the probability distribution, equation \eqref{eqn:p_r}, we can calculate the predicted mean velocity as, 
\begin{equation}
    \langle V_r \rangle = \int d r P(r|cz_{\text{obs}}) V_r(r)
\end{equation}
Similarly, we can calculate the standard deviation under the same probability distribution 
\begin{equation}
    \Delta V_{\text{pred}} = \left(\int d r P(r|cz_{\text{obs}}) (V_r(r)-\langle V_r \rangle)^2\right)^{1/2}
\end{equation}
which gives us an estimate of the uncertainty in the predicted velocity from reconstruction.

So far, we have considered a fixed reconstructed velocity field. In reality, the predicted velocity field has additional flow parameters, $\Theta = \{\beta, \mathbf{V}_{\text{ext}}\}$ which can be inferred by fitting to peculiar velocity data. The uncertainties in the inferred flow parameters can also lead to correlated uncertainties in the peculiar velocities which needs to be accounted for. In order to estimate this covariance, we take $10000$ samples of the flow parameters $\Theta$ inferred by fitting the parameters to the SFI++ peculiar velocity sample using the method of \citet{RN345}. We then calculate the predicted velocity, $\langle V_r \rangle$ for all the objects in the JLA catalogue. With the flow parameter sample, we then estimate the covariance of the predicted velocity, $C^{ij}_{\text{flow}} = \text{Cov}(V^i_r, V^j_r)$. 

We then add the additional velocity uncertainty, $\Delta V_r$ to the diagonal terms of this covariance. Note that we get an estimate of the velocity uncertainty, $\Delta V_r$ for all the flow parameter samples. The variation of $\Delta V_r$ for different samples in the MCMC chain is small ($< 10\%$) compared to its typical value. Hence, we take the mean value of $\Delta V_r$ estimated from the $10000$ MCMC samples for all the supernovae. We denote the covariance due to the reconstruction error as, $C^{ij}_{\text{rec}} = \Delta V^i_r \delta^{ij}_{K}$, where, $ \delta^{ij}_{K}$ is the Kronecker delta. 

Finally, we also need to account for the velocity uncertainty due to the non-linearities. We assume the velocity uncertainty in the predicted velocity due to the non-linearities to be the value, $\sigma_v=150$ km/s. We denote the covariance due to the non-linearities as, $\mathbf{C}_{\text{NL}} = \sigma^2_v \mathbf{I}$. 

The full covariance to account for the peculiar velocity uncertainty is therefore given as, 
\begin{equation}
    \mathbf{C} = \mathbf{C}_{\text{flow}} + \mathbf{C}_{\text{rec}} + \mathbf{C}_{\text{NL}}.
\end{equation}
